# Supplementary material for: Stress-driven whisker formation in lithium metal batteries
Source: arXiv:2503.21481 ancillary file (2025-03-27)
Supplement: Supplementary file 1 [file supporting_information_model_of_whisker_emergence.pdf]

## Supporting Information - Stress-driven whisker formation in lithium metal batteries

Martin Werres[1,2], Dariusz Niedziela[3], Arnulf Latz[1,2,4], and Birger Horstmann*[1,2,4]

Institute of Engineering Thermodynamics, German Aerospace Center (DLR), Wilhelm-Runge-Str. 10, 89081 Ulm, Germany

Helmholtz Institute Ulm (HIU), Helmholtzstr. 11, 89081 Ulm, Germany

Department Flow and Material Simulation, Fraunhofer Institute for Industrial Mathematics, Fraunhofer-Platz 1, D-67663 Kaiserslautern, Germany

Department of Electrochemistry, University of Ulm, Albert-Einstein-Allee 47, 89081 Ulm, Germany

### 1. Model Parameters

| Model parameters & physical constants | Value | Description |
|---|---|---|
| $D_{e^-}c_{e^-}$ | $1.5\times10^{-17}$ mol/m$^3$ | Diffusivity of electrons in SEI times concentration of electrons in the SEI near the Li interface |
| $V_m^{Li}$ | $13.02\times10^{-6}$ m$^3$/mol | Molar volume of Li |
| $V_m^{SEI}$ | $95.86\times10^{-6}$ m$^3$/mol | Molar volume of the SEI |
| $F$ | 96485 C/mol | Faraday constant |
| $C$ | $1.59\times10^{6}$ Pa s | Shear-thinning dimensionality constant |
| $n$ | 0.1515 | Stress exponent |
| $\sigma_{\text{yield}}$ | $1\times10^{7}$ Pa | Yield stress |
| $m$ | 100000 | Herschel-Bulkley regularization parameter |
| $\rho$ | 534 kg/m$^3$ | Lithium density |
| $\rho_{Electrolyte}$ | 1241 kg/m$^3$ | Electrolyte density |
| $\eta_{electrolyte}$ | $3.045\times10^{-3}$ Pa s | Electrolyte viscosity |

*SI Table 1: Table of model parameters and constants.*

The model parameters $C$ and $n$ are derived from the experimental observations of LePage et al. [1]. They observed that the secondary creep phase can be described by the power-law:

$$\frac{\dot{\epsilon}}{\mathrm{s}^{-1}} = A_c \left(\frac{\sigma}{\mathrm{Pa}}\right)^m \exp\left(-\frac{Q_c}{RT}\right),$$

where $\dot{\epsilon}$ is the strain rate, $\sigma$ is the uniaxial stress, and $m$, $A_c$, and $Q_c$ are material parameters determined by their experiments. They determined the coefficients to be $m = 6.6$, $A_c = 7.1 \times 10^{-37}$, and $Q_c = 37\ \mathrm{kJ\ mol^{-1}}$.

With this parameters, we can calculate an effective extensional viscosity $\mu_{\text{elongational}} = \sigma/\dot{\epsilon}$ :

$$\frac{\mu_{\text{elongational}}}{\mathrm{Pa\cdot s}} = \frac{\sigma}{\dot{\epsilon}} = A_c^{-\frac{1}{m}} \exp\left(\frac{Q_c}{mRT}\right)\left(\frac{\dot{\epsilon}}{s^{-1}}\right)^{\frac{1}{m}-1} .$$

At room temperature (T=293.15K), the elongational viscosity is:

$$\frac{\mu_{\text{elongational}}(T=293.15K)}{\text{Pa}\cdot\text{s}} = 2.99\times10^{6}\left(\frac{\dot{\epsilon}}{s^{-1}}\right)^{\frac{1}{m}-1}.$$

We make the assumption that the extensional viscosity can be related to the shear viscosity via the Trouton ratio:

$$Tr = \frac{\mu_{\text{elongational}}}{\mu_{\text{shear}}} \approx 3\,.$$

The shear rate is the second invariant of the strain-rate tensor:

$$\dot{\gamma} = \sqrt{2\epsilon:\epsilon}\,.$$

For $\epsilon = \begin{pmatrix} -0.5 & 0 & 0 \\ 0 & -0.5 & 0 \\ 0 & 0 & 1 \end{pmatrix}\dot{\epsilon}$, $\dot{\gamma} = \sqrt{3}\dot{\epsilon}$. We use this to express the shear viscosity as

$$\frac{\mu_{shear}}{\text{Pa}\cdot\text{s}} = \frac{1}{3}\cdot 3^{\frac{1-\frac{1}{m}}{2}}\cdot 2.99\times10^{6}\left(\frac{\dot{\gamma}}{s^{-1}}\right)^{\frac{1}{m}-1} = 1.59\times10^{6}\left(\frac{\dot{\gamma}}{s^{-1}}\right)^{\frac{1}{m}-1}.$$

Thus, the model parameters are $C = 1.59\times10^{6}\ \text{Pa}\cdot\text{s}$ and $n = \frac{1}{m} = 0.1515$.

## 2. Detailed Setup

The simulation domain is setup with

$$\Delta x = \Delta y = \Delta z = 10\ \text{nm}$$

and a cross-section of the simulation domain is shown in Figure SI 1. The white space is void and not solved for. The parts of the simulation domain which don’t have a connection to a different domain are  bounded by no-slip wall conditions.

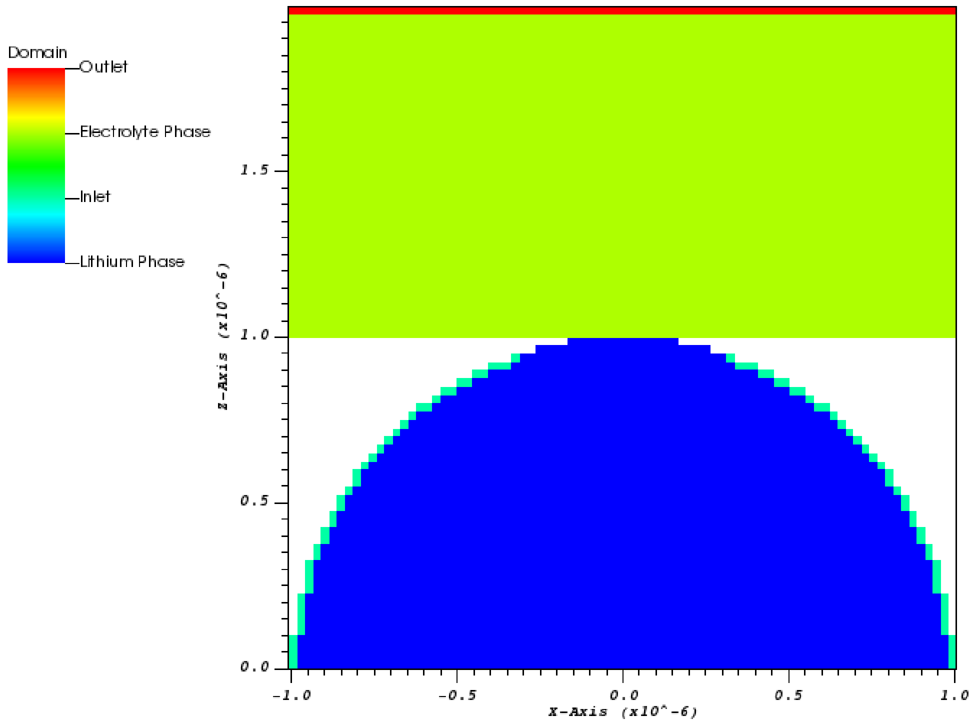


*SI 2: Cross-section of the simulation domain setup. The initial Herschel-Bulkley phase is blue, the inlet is turquoise, the electrolyte phase is green, and the outlet is red.*

## 3. Impact of yield stress on pressure distribution

Since we can only estimate the yield stress of Lithium on this small length scales, we studied how the predicted pressure distribution changes for a different yield stress. The bulk yield stress of lithium is reported to be between 0.57 and 1.26 MPa, we chose 1 MPa as a comparison. The resulting pressure distribution is depicted in Figure SI 2. Comparing this to the results with $\sigma_{yield}$ =10 MPa, the stress distribution looks similar but the predicted pressure values are overall smaller by a factor of approximately 3.

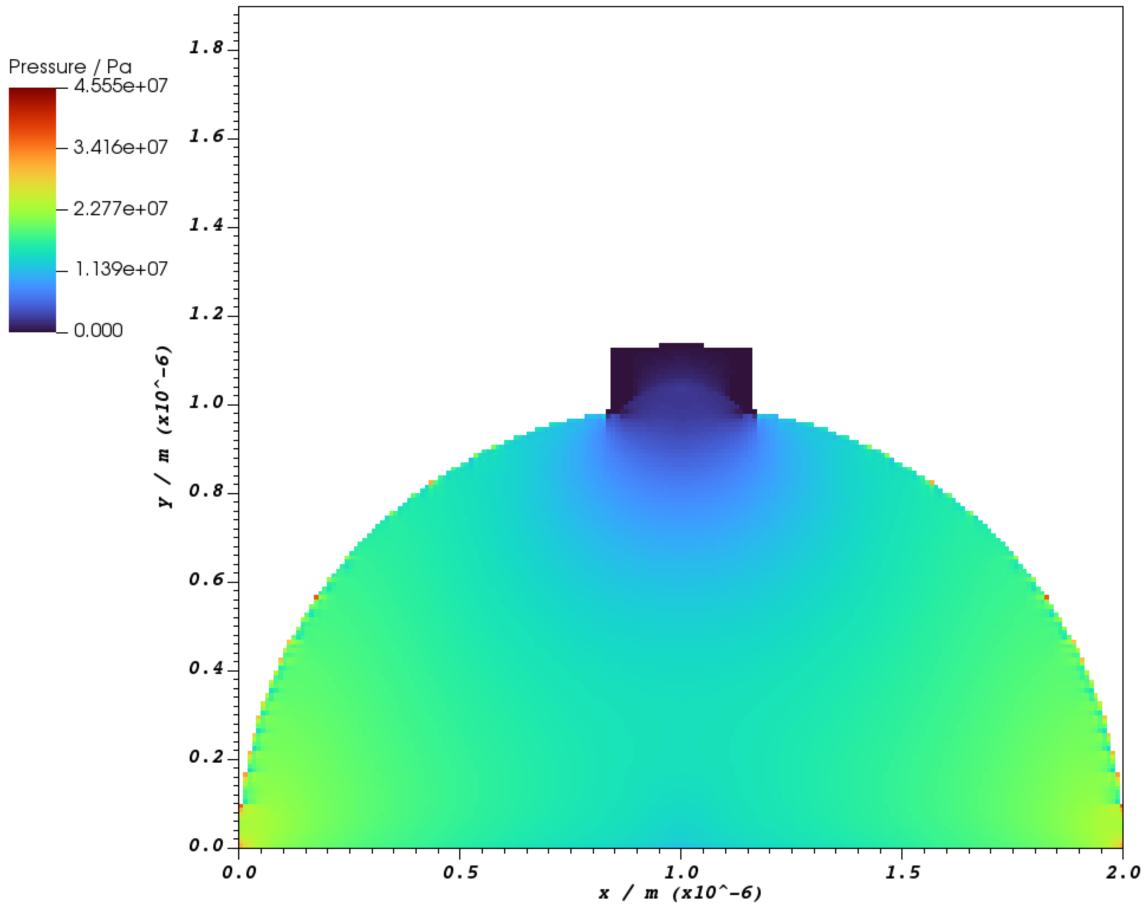


*SI 3: Predicted pressure distribution with yield stress = 1 MPa, after t = 0.15s.*

## References

[1] LePage, W. S. *et al.* Lithium Mechanics: Roles of Strain Rate and Temperature and Implications for Lithium Metal Batteries. *J. Electrochem. Soc.* **166**, A89–A97 (2019)
